# Supplementary material for: Fooling Polarization-based Vision using Locally Controllable Polarizing Projection
Source: arXiv:2303.17890 source file (2024-06-19)
Supplement: Supplementary file 2 [file supp.pdf]

# Fooling Polarization-based Vision using Locally Controllable Polarizing Projection

## Supplementary Material

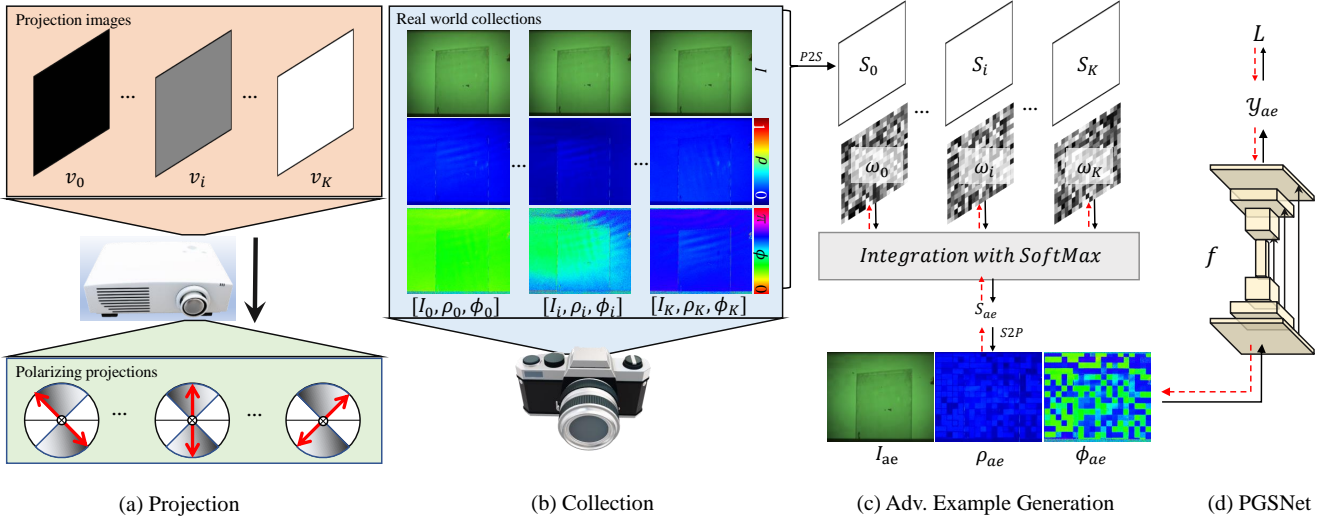

Figure 1. Illustrations of (a) polarizing projections, (b) candidate images collection, (c) adversarial example generation, and (d) feed forward & gradient backward of the polarization-RGB-based glass segmentation model PGSNet [6].  $v_i$  represents the pixel value for the projected monochromatic image.  $[I_i, \rho_i, \phi_i]$  denote captured polarization cues, including intensity, DoLP, and AoLP maps, and  $S_i$  are the same data in the form of Stokes parameters.  $S2P$  and  $P2S$  represent conversions between Polarization cues and Stokes parameters. Black and red dashed lines in (c), (d) counts for flows of data feed-forward and gradients backward propagation.

## 1. Whitebox Attack on Glass Segmentation

### 1.1. Implementation Details

We propose to employ locally controllable polarizing projection to fool the polarization-RGB-based glass segmentation model, PGSNet [6], in the physical world. We control the polarizing projection by projecting specific images according to the principle of our adapted one-chip LCD projector. In general, physical world adversarial attacks require realistic simulations of targeted objects as well as scenes injected with adversarial perturbations, *e.g.*, projection [4], shadow [8], and stickers [3], to search a robust and effective adversarial perturbation pattern. However, polarization reflection modeling requires accurate pBRDF parameters [2] and geometries that are unavailable in the wild. Thus, we propose a simplified approach for constructing a simulation of high precision.

Our perturbation is a map of grids, and pixels in each grid are assigned a same value to construct a perturbation robust enough to be captured in the complex real world. The adversarial perturbation should be estimated in an optimization-based approach in whitebox attack. To avoid physics-based simulation of polarized light transports from the projector to the camera, which involves the non-linear function of the projector and polarization reflection modeling, we generate adversarial examples from a set of candidate real captures whose projection values are known.

Concretely, we first set the projector (ELEPHAS W13 after hardware modification) and RGB-P camera (BFS-U3-51S5PC-C equipped with the IMX250MYR Polar-RGB sensor) in the same place and both look forward to the target scene. Then, we project flat grayscale images of a gray level  $\{v_0, \dots, v_K\}$  uniformly sampled from 0 to 255, which causes projections with constant polarizing directions, as

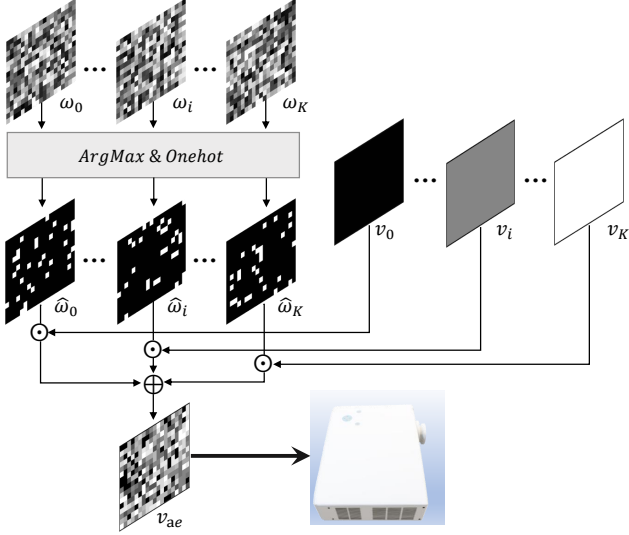

Figure 2. The illustration of generating final projection perturbation image. The optimized weights  $\Omega = \{\omega_0, \dots, \omega_K\}$  is processed by the *ArgMax* function and converted into one-hot maps as  $\hat{\omega}_i$ , and finally integrated into the ultimate projection perturbation image  $v_{ae}$ .

shown in Figure 1 (a). Next, we capture a sequence of real-world images as a set of bases. As shown in Figure 1 (b) in the form of polarization cues, in contrast to few differences between the intensity images  $I_i$ , their AoLP maps  $\phi_i$  are significantly changed by polarizing projections. In Figure 1 (c), the basis images in the form of Stokes parameters are integrated into  $S_{ae}$  with a set of optimizable weight maps  $\Omega = \{\omega_0, \dots, \omega_{pk}\}$  through the *SoftMax* function as:

$$S_{ae} = \sum_i^K \frac{\exp(\omega_i/\tau)}{\sum_j^K \exp(\omega_j/\tau)} (S_i - S_b) + S_b^*, \quad (1)$$

where  $S_b$  denotes the Stokes parameter of background and  $S_b^*$  is that rescaled for augmentation. The integration  $[I_{ae}, \rho_{ae}, \phi_{ae}]$  is fed into PGSNet as an adversarial example, to optimize the coefficient maps  $\Omega$ , as shown in Figure 1 (d).

After the optimization, the best projection value in each grid is selected from  $\{v_0, \dots, v_K\}$  by *ArgMax* function. As shown in Figure 2,  $v_{ae}$  is our final perturbation image for polarizing projection. The proposed approach generates adversarial examples and optimizes the perturbation from real images, thus achieving high effectiveness in the physical world attack.

## 1.2. Adversarial Loss

The total loss function consists of a BCE loss and  $L_E$ . We want to mislead the PGSNet to predict more negative pixels to be positive, and on the opposite predict more positive pixels to be negative as [5]. Thus, with the prediction

of adversarial example  $y_{ae}$ ,  $L_E$  is termed as:

$$\mathcal{L}_E = \frac{1}{HW} \sum_{j \in y^n} y_{ae}^j - \frac{1}{HW} \sum_{j \in y^p} y_{ae}^j, \quad (2)$$

where  $y^{\{n,p\}}$  denotes the set of pixels which are negative / positive (not-glass / glass) in the label  $y$ .  $y^n$  and  $y^p$  are disjoint, and the total number of pixels of  $y^n \cup y^p$  is  $HW$ .

## 1.3. Experiment

We show more visual results of physical world attacks. As shown in Figure 3, compared with unpolarized illumination (Unp.) or random perturbations (in the sub-pictures), our optimized polarizing projections achieve effective and robust adversarial attacks in the physical world. For scene 3 (a), random perturbation is sufficient to mislead the PGSNet while the background wall is glossy and the edge of the glass is not distinct enough. But randomly sampled perturbations fail in a more complicated scene (b), in which the glass has clear edges and prominent polarization cues. In contrast, our adversarial projection perturbation is optimized in a whitebox manner with simulating real-world degradations, thus can deal with such complex cases.

## 2. Blackbox Attack on Color Constancy

### 2.1. Implementation Details

The DoLP-based color constancy algorithm [7] estimates white-balance ratios from channel-wise polarization cues, DoLP principally. Thus, we simply project empty colorful images, which represent color-wise polarizing projections, to misguide the restoration. Note that, since our LCD projector has three (R, G, B) independent color channels, the polarization direction of each color channel can be controlled individually. We utilize this color-wise flexibility for fooling color constancy, with uniform value in each color channel of the projection image. As shown in Figure 4 (a), while we project an empty image filled with red ( $[255, 0, 0]$  in 3 channels) to the target scene, our polarizing projector projects constant white light, of which RGB components are linearly polarized in individual directions. The original raw image  $I_{ori}$  in (a) is slightly green even under white illumination, since the automatic white balance mode of the camera is switched off. We can also employ an additional color filter before the projector to further modify the illumination color, as shown in Figure 4 (b), which usually makes color constancy more challenging.

## References

- [1] Anish Athalye, Logan Engstrom, Andrew Ilyas, and Kevin Kwok. Synthesizing robust adversarial examples. In *International conference on machine learning*, pages 284–293. PMLR, 2018. 3

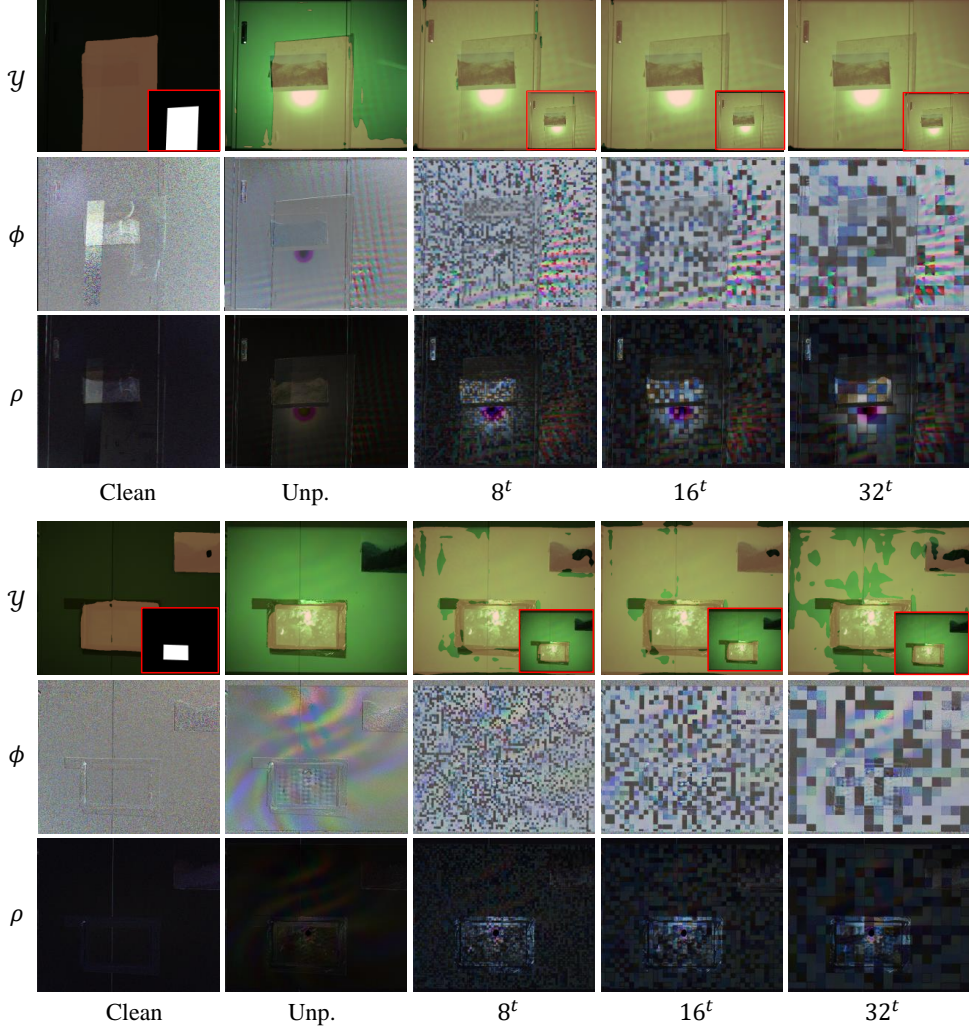

Figure 3. Visual comparisons for adversarial attacks on the polarization-based glass segmentation model PGsNet [6] in the physical world.  $y$ ,  $\phi$  and  $\rho$  represent predictions, AoLP, and DoLP maps respectively. The orange denotes regions predicted as glass pixels. Clean shows background images caused by environment lighting, without any projections. Unp. denotes scenes illuminated by unpolarized light. 8, 16 and 32 represent grid sizes and  $*^t$  denotes perturbations optimized with simulated real-world disturbances [1]. The sub-pictures in red square in Clean show labels and the others show predictions with randomly generated perturbations in the corresponding grid sizes.

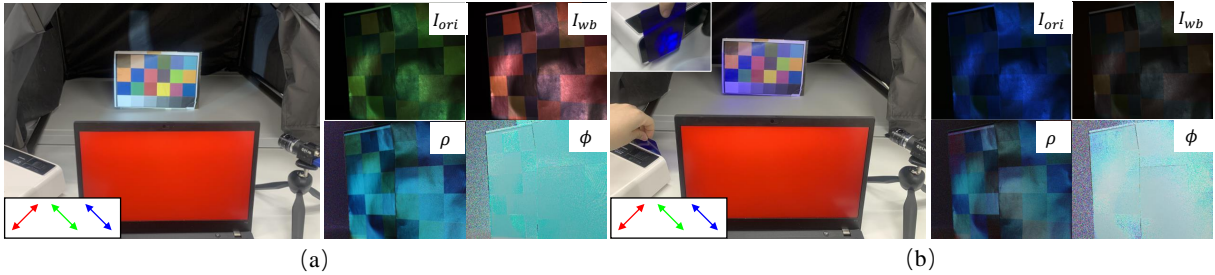

Figure 4. Illustrations for blackbox attacks on DoLP-based color constancy using color-wise polarizing projections. (a) and (b) are scenes w/o and w/ an additional color filter before the projector. The connected computer controls the polarizing projector by projecting an image, e.g., a red image. Note that, although the projection image is red, the projected light is uniform white to human eyes (a). After going through an additional blue filter, the light looks blueish to human eyes (b). The polarization direction of emitted color-wise polarizing projection is illustrated in the left-bottom in (a), (b).  $I_{ori}$ ,  $\rho$ ,  $\phi$  are intensity, DoLP, and AoLP maps, and  $I_{wb}$  is the restoration result.

- [2] Seung-Hwan Baek, Daniel S Jeon, Xin Tong, and Min H Kim. Simultaneous acquisition of polarimetric svbrdf and normals. *ACM Trans. Graph.*, 37(6):268–1, 2018. [1](#)
- [3] Kevin Eykholt, Ivan Evtimov, Earlence Fernandes, Bo Li, Amir Rahmati, Chaowei Xiao, Atul Prakash, Tadayoshi Kohno, and Dawn Song. Robust physical-world attacks on deep learning visual classification. In *Proceedings of the IEEE conference on computer vision and pattern recognition*, pages 1625–1634, 2018. [1](#)
- [4] Abhiram Gnanasambandam, Alex M Sherman, and Stanley H Chan. Optical adversarial attack. In *Proceedings of the IEEE/CVF International Conference on Computer Vision*, pages 92–101, 2021. [1](#)
- [5] Jindong Gu, Hengshuang Zhao, Volker Tresp, and Philip HS Torr. Segpgd: An effective and efficient adversarial attack for evaluating and boosting segmentation robustness. In *Computer Vision–ECCV 2022: 17th European Conference, Tel Aviv, Israel, October 23–27, 2022, Proceedings, Part XXIX*, pages 308–325. Springer, 2022. [2](#)
- [6] Haiyang Mei, Bo Dong, Wen Dong, Jiayi Yang, Seung-Hwan Baek, Felix Heide, Pieter Peers, Xiaopeng Wei, and Xin Yang. Glass segmentation using intensity and spectral polarization cues. In *Proceedings of the IEEE/CVF Conference on Computer Vision and Pattern Recognition*, pages 12622–12631, 2022. [1](#), [3](#)
- [7] Taishi Ono, Yuhi Kondo, Legong Sun, Teppei Kurita, and Yusuke Moriuchi. Degree-of-linear-polarization-based color constancy. In *Proceedings of the IEEE/CVF Conference on Computer Vision and Pattern Recognition*, pages 19740–19749. IEEE, 2022. [2](#)
- [8] Yiqi Zhong, Xianming Liu, Deming Zhai, Junjun Jiang, and Xiangyang Ji. Shadows can be dangerous: Stealthy and effective physical-world adversarial attack by natural phenomenon. In *Proceedings of the IEEE/CVF Conference on Computer Vision and Pattern Recognition*, pages 15345–15354, 2022. [1](#)
